# Supplementary material for: Logic-based Benders Decomposition and Binary Decision Diagram Based Approaches for Stochastic Distributed Operating Room Scheduling
Source: arXiv:1907.13265 source file (2020-10-02)
Supplement: Supplementary file 1 [file SDORS_OnlineSupplement.tex]

%%%%%%%%%%%%%%%%%%%%%%%%%%%%%%%%%%%%%%%%%%%%%%%%%%%%%%%%%%%%%%%%%%%%%%%%%%%%
%% Author template for INFORMS Journal on Computing (ijoc)
%% Mirko Janc, Ph.D., INFORMS, mirko.janc@informs.org
%% ver. 0.95, December 2010
%%%%%%%%%%%%%%%%%%%%%%%%%%%%%%%%%%%%%%%%%%%%%%%%%%%%%%%%%%%%%%%%%%%%%%%%%%%%
%\documentclass[ijoc,blindrev]{informs3}
\documentclass[ijoc,nonblindrev]{informs3} % current default for manuscript submission

%%\OneAndAHalfSpacedXI
\OneAndAHalfSpacedXII % current default line spacing
%%\DoubleSpacedXII
%%\DoubleSpacedXI

% If hyperref is used, dvi-to-ps driver of choice must be declared as
%   an additional option to the \documentclass. For example
%\documentclass[dvips,ijoc]{informs3}      % if dvips is used
%\documentclass[dvipsone,ijoc]{informs3}   % if dvipsone is used, etc.

% Private macros here (check that there is no clash with the style)

% Natbib setup for author-year style
\usepackage{natbib}
 \bibpunct[, ]{(}{)}{,}{a}{}{,}%
 %
 %
 %
 %
 %

%% Setup of theorem styles. Outcomment only one. 
%% Preferred default is the first option.
\TheoremsNumberedThrough     % Preferred (Theorem 1, Lemma 1, Theorem 2)
%\TheoremsNumberedByChapter  % (Theorem 1.1, Lema 1.1, Theorem 1.2)

%% Setup of the equation numbering system. Outcomment only one.
%% Preferred default is the first option.
\EquationsNumberedThrough    % Default: (1), (2), ...
%\EquationsNumberedBySection % (1.1), (1.2), ...

% In the reviewing and copyediting stage enter the manuscript number.
%\MANUSCRIPTNO{} % When the article is logged in and DOI assigned to it,
                 %   this manuscript number is no longer necessary

\include{Definitions}
\usepackage{xr}
\externaldocument{SDORS_JOC_paper}
%%%%%%%%%%%%%%%%
\begin{document}
%%%%%%%%%%%%%%%%

% Outcomment only when entries are known. Otherwise leave as is and 
%   default values will be used.
%\setcounter{page}{1}
%\VOLUME{00}%
%\NO{0}%
%\MONTH{Xxxxx}% (month or a similar seasonal id)
%\YEAR{0000}% e.g., 2005
%\FIRSTPAGE{000}%
%\LASTPAGE{000}%
%\SHORTYEAR{00}% shortened year (two-digit)
%\ISSUE{0000} %
%\LONGFIRSTPAGE{0001} %
%\DOI{10.1287/xxxx.0000.0000}%

% Author's names for the running heads
% Sample depending on the number of authors;
% \RUNAUTHOR{Jones}
% \RUNAUTHOR{Jones and Wilson}
% \RUNAUTHOR{Jones, Miller, and Wilson}
% \RUNAUTHOR{Jones et al.} % for four or more authors
% Enter authors following the given pattern:
%\RUNAUTHOR{}

% Title or shortened title suitable for running heads. Sample:
% \RUNTITLE{Bundling Information Goods of Decreasing Value}
% Enter the (shortened) title:
%\RUNTITLE{}

% Full title. Sample:
% \TITLE{Bundling Information Goods of Decreasing Value}
% Enter the full title:
%\TITLE{}

% Block of authors and their affiliations starts here:
% NOTE: Authors with same affiliation, if the order of authors allows, 
%   should be entered in ONE field, separated by a comma. 
%   \EMAIL field can be repeated if more than one author

\RUNAUTHOR{Guo et. al.}

% Title or shortened title suitable for running heads. Sample:
% \RUNTITLE{Bundling Information Goods of Decreasing Value}
% Enter the (shortened) title:
\RUNTITLE{Online Supplement ``LBBD and BDD Based Approaches for SDORS"}

% Full title. Sample:
% \TITLE{Bundling Information Goods of Decreasing Value}

% Enter the full title:
%\title{Split Cuts for Stochastic Integer Programming%\thanks{Grants or other notes
%about the article that should go on the front page should be
%placed here. General acknowledgments should be placed at the end of the article.}
%}
\TITLE{Online Supplement for ``Logic-based Benders Decomposition and Binary Decision Diagram Based Approaches for Stochastic Distributed Operating Room Scheduling"}
%\title{Integrality-enhanced Benders Decomposition for Stochastic Integer Programming}
%% Jim: Still not sure of title, we could describe the things more generally as
%Benders decomposition in which the non-projected variables are integral (the
%typical case for "classic" Benders decomposition in IP), or focus on the
%stochastic programming case...
% Even if we describe it for Benders generically, we would still definitely
% highlight stochastic integer programming as the primary motivation

% Block of authors and their affiliations starts here:
% NOTE: Authors with same affiliation, if the order of authors allows, 
%   should be entered in ONE field, separated by a comma. 
%   \EMAIL field can be repeated if more than one author
\ARTICLEAUTHORS{%
\AUTHOR{Cheng Guo, Merve Bodur}
\AFF{Department of Mechanical and Industrial Engineering, University of Toronto, Toronto, Ontario M5S 3G8, Canada, \EMAIL{cguo@mie.utoronto.ca}, \EMAIL{bodur@mie.utoronto.ca}}
\AUTHOR{Dionne M. Aleman}
\AFF{Department of Mechanical and Industrial Engineering, University of Toronto, Toronto, Ontario M5S 3G8, Canada}
\AFF{Institute of Health Policy, Management and Evaluation, University of Toronto, Toronto, Ontario M5S 3E3, Canada}
\AFF{Techna Institute at University Health Network, Toronto, Ontario M5G 1P5, Canada, \EMAIL{aleman@mie.utoronto.ca}}
\AUTHOR{David R. Urbach}
\AFF{Techna Institute at University Health Network, Toronto, Ontario M5G 1P5, Canada}
\AFF{Department of Surgery, Women's College Hospital, Toronto, Ontario M5S 1B2, Canada, 
\EMAIL{david.urbach@wchospital.ca}}
}

\ABSTRACT{%
This supplement document provides all appendices referenced in the body of the paper.
%Given an integer dimension $\K$ and a simple, undirected graph $\graph$ with positive edge weights, the Distance Geometry Problem (DGP) aims to find a realization function mapping each vertex to a coordinate in $\R^\K$ such that the distance between pairs of vertex coordinates is equal to the corresponding edge weights in $\graph$. The so-called discretization assumptions reduce the search space of the realization to a finite discrete one, which can be explored via the branch-and-prune (BP) algorithm. Given a \emph{discretization vertex order} in $\graph$, the BP algorithm constructs a binary tree where the nodes at a layer provide all possible coordinates of the vertex corresponding to that layer. The focus of this paper is finding \emph{optimal BP trees} for a class of Discretizable DGPs. More specifically, we aim to find a discretization vertex order in $\graph$ that yields a BP tree with the least number of branches. We propose an integer programming formulation and three constraint programming formulations that all significantly outperform the state-of-the-art cutting plane algorithm for this problem. Moreover, motivated by the difficulty in solving instances with a large and low density input graph, we develop two hybrid decomposition algorithms, strengthened by a set of valid inequalities, which further improve the solvability of the problem.
}%
%
%% Sample 
%%\KEYWORDS{deterministic inventory theory; infinite linear programming duality; 
%%  existence of optimal policies; semi-Markov decision process; cyclic schedule}
%
%% Fill in data. If unknown, outcomment the field
%\KEYWORDS{Distance geometry; discretization order; integer programming; constraint programming; decomposition algorithms}
%%\HISTORY{}

\maketitle
%%%%%%%%%%%%%%%%%%%%%%%%%%%%%%%%%%%%%%%%%%%%%%%%%%%%%%%%%%%%%%%%%%%%%%

% Samples of sectioning (and labeling) in IJOC
% NOTE: (1) \section and \subsection do NOT end with a period
%       (2) \subsubsection and lower need end punctuation
%       (3) capitalization is as shown (title style).
%
%\section{Introduction.}\label{intro} %%1.
%\subsection{Duality and the Classical EOQ Problem.}\label{class-EOQ} %% 1.1.
%\subsection{Outline.}\label{outline1} %% 1.2.
%\subsubsection{Cyclic Schedules for the General Deterministic SMDP.}
%  \label{cyclic-schedules} %% 1.2.1
%\section{Problem Description.}\label{problemdescription} %% 2.

% Text of your paper here
%\input{Intro}
%\input{Prelim}
%\input{Models}
%\input{Hybrid}
%\input{Results}
%\input{Conclusion}

% Acknowledgments here
%\ACKNOWLEDGMENT{%
% Enter the text of acknowledgments here
%}% Leave this (end of acknowledgment)

% Appendix here
% Options are (1) APPENDIX (with or without general title) or 
%             (2) APPENDICES (if it has more than one unrelated sections)
% Outcomment the appropriate case if necessary
%
% \begin{APPENDIX}{<Title of the Appendix>}
% \end{APPENDIX}
%
%   or 
%

%\begin{APPENDICES}
\input{AppendProof}
\section{Simple Example for BDD}\label{chapter: app_example}
The following simple example provides an illustration of the BDD transformation. Suppose in {\cred the subproblem \eqref{model: sors_sub}} for an $(h, d, r, s)$ tuple there are four scheduled patients, and we need to decide whether to cancel them. The subproblem formulation is the following {\cred (we have replaced all $\hat{x}_{hdp}, p =1,...,4$ in subproblem \eqref{model: sors_sub} with 1, as all four patients are selected)}:
\begin{align*}
{\cred \bar{Q}_{hdr}^s = \min} \ & 4(1 - z^s_{hd1r})+(1- z^s_{hd2r})+3(1- z^s_{hd3r})+8(1-z^s_{hd4r}) &&\\
\text{s.t.} \ & {\cred 2z^s_{hd1r}+z^s_{hd2r}+3z^s_{hd3r}+3z^s_{hd4r} \leq 5}&& \\
&z^s_{hdpr}  \leq 1 &&\forall p\in\hat{\mc{P}}_{hdr}\\
& z^s_{hdpr} \in \{0,1\} &&\forall p\in\hat{\mc{P}}_{hdr}
\end{align*}
where $\hat{\mc{P}}_{hdr} = \{1,2,3,4\}$ {\cred represents the subset of selected patients. To simplify the notation, we equivalently rewrite the objective as:} 
\begin{align*}
{\cred \bar{Q}_{hdr}^s - 16 = \min~~ - 4z^s_{hd1r} - z^s_{hd2r} - 3z^s_{hd3r} - 8z^s_{hd4r}}
\end{align*}

The problem is reformulated via the BDD in Figure \ref{fig: bdd_example}. The BDD contains a root node at the top, denoted by $o$, and a terminal node at the bottom, denoted by $t$. Each layer of the arcs represents the values of the variables $z^s_{hdpr}$, from patient 1 to patient 4. Notice that the patients can be sorted in a different way from the order in the graph, and that will produce a different BDD, thus may result in different computational performance. At each layer, the dashed and solid arcs respectively indicate selecting 0 and 1 values for the layer's corresponding variable. The value above or beside each arc is the cost of $z^s_{hdpr}$ if it receives the value indicated by the arc type. When transferring the subproblem to a shortest path problem, those values are used as costs for the arcs. Each route from the node $o$ to the node $t$ represents a feasible solution for the subproblem, and each feasible solution is represented by a route from the node $o$ to the node $t$. Also, the path length provides the correct evaluation of the objective value for a corresponding feasible solution. Therefore, by finding a shortest path from the root node to the terminal node, we are able to obtain an optimal solution to the subproblem. 

\begin{figure}[h]
\centering
\begin{tikzpicture}[scale=0.3][font=\sffamily,\tiny]
	\tikzset{mycircle/.style={draw,circle, minimum size=0.4cm}}
	\tikzstyle{arrow} = [thick,->,>=stealth]

	\node [mycircle] (r) at (0,0) {$o$};

	\node [mycircle,left of=r,xshift=-0.3cm,yshift=-1cm] (a)  {$a$};
	\node [mycircle,right of=r,xshift=0.3cm,yshift=-1cm] (b) {$b$};

	\node [mycircle,below of=a,yshift=-0.4cm] (c)  {$c$};
	\node [mycircle,below of=b,yshift=-0.4cm] (d) {$d$};

	\node [mycircle,below of=c,yshift=-0.4cm] (e)  {$e$};
	\node [mycircle,below of=d,yshift=-0.4cm] (f) {$f$};

	\node [mycircle] at ([yshift=-3.2cm]e -| r) (t) {$t$} ;

	\node [left of=a,xshift=-1cm,yshift=0.7cm,scale=1.2] (x1) {$z^s_{hd1r}$};
	\node [left of=a,xshift=-1cm,yshift=-0.7cm,scale=1.2] (x2) {$z^s_{hd2r}$};
	\node [left of=c,xshift=-1cm,yshift=-0.7cm,scale=1.2] (x3) {$z^s_{hd3r}$};
	\node [left of=e,xshift=-1cm,yshift=-0.7cm,scale=1.2] (x4) {$z^s_{hd4r}$};

	\draw[arrow,dashed] (r) -- node[anchor=south,xshift = -0.35cm,yshift=-0.1cm,scale=1.3] {0} (a);
	\draw[arrow] (r) -- node[anchor=south,xshift = 0.35cm,yshift=-0.1cm,scale=1.3] {$- 4$} (b);%c^{\text{cancel}}_1

	\draw[arrow,dashed] (a) [bend left] to node[anchor=south,xshift = 0.2cm,yshift=-0.1cm,scale=1.3] {0} (c);
	\draw[arrow] (a) [bend right] to node[anchor=south,xshift = -0.4cm,yshift=-0.1cm,scale=1.3] {$- 1$} (c);

	\draw[arrow,dashed] (b) -- node[anchor=south,xshift = 0.3cm,yshift=0.3cm,scale=1.3] {0} (c);
	\draw[arrow] (b) -- node[anchor=south,xshift = 0.35cm,yshift=-0.1cm,scale=1.3] {$- 1$} (d);
	\draw[arrow] (c) -- node[anchor=south,xshift = 0.1cm,yshift=0.1cm,scale=1.3] {$- 3$} (f);
	\draw[arrow,dashed] (c) -- node[anchor=south,xshift = -0.3cm,yshift=-0.1cm,scale=1.3] {0} (e);
	\draw[arrow,dashed] (d) -- node[anchor=south,xshift = 0.3cm,yshift=-0.1cm,scale=1.3] {0} (f);
	\draw[arrow,dashed] (f) -- node[anchor=south,xshift = 0.3cm,yshift=-0.4cm,scale=1.3] {0}(t);

	\draw[arrow,dashed] (e) [bend left] to node[anchor=south,xshift = 0.1cm,yshift=0cm,scale=1.3] {0} (t);
	\draw[arrow] (e) [bend right] to node[anchor=south,xshift = -0.5cm,yshift=-0.23cm,scale=1.3] {$- 8$} (t);
\end{tikzpicture}
\caption{BDD for a simple subproblem with four patients}
\label{fig: bdd_example}
\end{figure}
%\newpage
%--%
\section{Flow Chart for the Two-stage Decomposition}\label{chapter: app_flowchart}
\begin{figure}[H] 
%\FIGURE
\begin{center}
%\vspace*{0.3cm}
{
\begin{tikzpicture}[node distance=1.75cm]
\tikzstyle{startstop} = [rectangle, rounded corners, minimum width=1.15cm, minimum height=0.7cm,text centered, draw=black, fill = gray!40!white]
%fill=red!30
%\tikzstyle{io} = [trapezium, trapezium left angle=70, trapezium right angle=110, minimum width=3cm, minimum height=1cm, text centered, draw=black, fill=blue!30]
%\tikzstyle{process} = [rectangle, minimum width=3cm, minimum height=1cm, text centered, draw=black, fill=orange!30]
\tikzstyle{process} = [rectangle, minimum width=2cm, minimum height=1cm, text centered, text width=1.98cm, draw=black]
\tikzstyle{decision} = [diamond, aspect=1.4, text centered, text width=1.2cm, draw=black]
\tikzstyle{arrow} = [thick,->,>=stealth]
\small
\node (start) [startstop] {START};
\node (lp1) [process, right of=start,xshift = 0.7cm,text width=2.5cm] {Add adapted FFD heuristic solution as MIP start};
\node (ben1) [process, right of=lp1,xshift = 1.2cm,text width=1.8cm] {Generate cuts from heuristic solution};
\node (vio1) [process, right of=ben1,xshift = 1.2cm,text width=2.5cm] {Generate\\ constraints from subproblem relaxation};
%\node (vio1) [decision, right of=ben1,aspect=1.2,xshift = 1.25cm] {Violated cuts?};
%\node (dummy1) [above of=vio1, yshift = -0.2cm] {};

\node (trans) [process, right of=vio1,text width=4cm,xshift = 2.5cm] {Add cuts and constraints \\ from Phase one to initial master formulation in Phase two};
\node (dummytrans) [xshift = -1cm] at (trans.south) {};

\node (stopping) [decision, below of=dummytrans,aspect=1.2,yshift = -3.85cm, text width=1.47cm] {Stopping criterion?};
\node (stop) [startstop, right of=stopping,xshift = 1.5cm] {STOP};
%\node (snode) [process,text width=1.5cm,fill = gray!10!white] at (vio1 |- stopping) {Select/ remove node};
\node (lp2) [process,text width=2.2cm] at (vio1 |- stopping) {Solve node LP relaxation};

\node (vio2) [decision, above of=lp2,aspect=1.2,yshift = 1.2cm] {$\hat{Q} < \bar{Q}$ or $\hat{Q} < \bar{Q}^{\text{LP}}$?};
\node (vio3) [decision, below of=lp2,aspect=1.2,yshift = -1.1cm] {$\hat{Q} < \bar{Q}^{\text{LP}}$?};

%\node (branch) [process,text width=1.5cm,fill = gray!10!white] at (vio2 -| snode) {Create branches};
%\node (ub) [process,text width=1.5cm] at (vio3 -| snode) {Update UB};

\node (ben2) [process,text width=3.5cm] at (lp1.east |- vio2) {Generate LBBD / BDD-based Benders cuts and Classical \\Benders cuts};
\node (ben3) [process,text width=2.5cm] at (lp1 |- vio3) {Generate Classical Benders cuts};

\node (UBheur) [process,left of=ben2,xshift= -1.8cm,text width=1.5cm, text centered] {Apply heuristic callback};

\node (check) [decision, aspect=1.33,text width=1.4cm ,left of=lp2,xshift= -5cm] {Check \\ integrality};
\node (dummycheck1) [left of=check, xshift=-0.4cm] {};
\node (dummyinf) [left of=check, xshift=-0.48cm] {};
\node (dummycheck2) [below of=dummyinf, yshift=-2.6cm] {};
\node (dummy3) [right of=vio3, xshift=0.35cm] {};

\draw [arrow] (start) -- (lp1);
\draw [arrow] (lp1) -- (ben1);
\draw [arrow] (ben1) -- (vio1);
%\draw [-,thick] (vio1) -- node[anchor=south,xshift = 0.32cm,yshift=-0.27cm] {yes} (dummy1);
%\draw [arrow] (dummy1.south) -| (lp1);
\draw [arrow] (vio1) -- (trans);
\draw [arrow] (dummytrans.center) -- (stopping);
\draw [arrow] (stopping) -- node[anchor=east,xshift = 0.2cm,yshift=0.2cm] {Yes} (stop);
\draw [arrow] (stopping) -- node[anchor=south,xshift = 0.1cm,yshift=0.01cm] {No} (lp2);
%\draw [arrow] (snode) -- (lp2);

\draw [arrow] (vio2) -- node[anchor=south,xshift = 0.32cm,yshift=-0.1cm] {Yes} (lp2);
\draw [arrow] (vio3) -- node[anchor=south,xshift = 0.32cm,yshift=-0.36cm] {Yes} (lp2);

%\draw [arrow] (vio2) -- node[anchor=south,xshift = -0.1cm,yshift=-0.01cm] {no} (branch);
%\draw [arrow] (vio3) -- node[anchor=north,xshift = -0.1cm,yshift=0.01cm] {no} (ub);

\draw [arrow] (vio2) -- node[anchor=south,xshift = -0.6cm,yshift=-0.01cm] {No} (vio2 -| stopping);
\draw [arrow] (vio3) -| node[anchor=north,xshift = -1 cm,yshift=0.01cm] {No} (stopping);

\draw [arrow] (ben2) -- (vio2);
\draw [arrow] (ben3) -- (vio3);

\draw [arrow] (UBheur) -- (ben2);

\draw [arrow] (lp2) -- (check);
%\draw [arrow] (check.west) -- node[anchor=west,text width=1.8cm,xshift = 0cm,yshift=0.6cm] {($\nu < \text{UB}$) \\ and $\bar{z} \notin \Zplus^{\Icard \Scard}$} (UBheur.south -| check.west);
%\draw [arrow] (check.west) |- node[anchor=west,text width=1.8cm,xshift = 0cm,yshift=0.5cm] {($\nu < \text{UB}$) \\ and  $\bar{z} \in \Zplus^{\Icard \Scard}$} (ben3);
\draw [arrow] (dummycheck1.center) -- node[anchor=west,text width=1.85cm,xshift = 0cm,yshift=0.4cm] {$(\hat{u}, \hat{y}, \hat{x}, \hat{w})$ is integral } (UBheur.south -| dummycheck1.center);%\usepackage{tikz}
\draw [arrow] (check.south) -- node[anchor=west,text width=2.3cm,xshift = 0cm,yshift=0.12cm] {$(\hat{u}, \hat{y}, \hat{x}, \hat{w})$ is not integral} (check.south |- ben3.north);% \in \Zplus^{\Icard \Scard}$

\draw [-,thick] (check) -- (dummycheck1.center);
%\draw [-,thick] (dummyinf.center) -- node[anchor=west,text width=4cm,xshift = 0cm,yshift=-1.9cm] {($\nu \geq \text{UB})$ or Infeasible} (dummycheck2.center);
%\draw [arrow] (dummycheck2.center) -| (dummy3.center);

\node [thick,xshift=0.15cm,draw=black,rounded corners=2mm, dotted, minimum width=9.1cm, minimum height=0.1cm, fit = (lp1) (vio1) ] (Phase1)  {};
\node [thick,xshift=0.27cm,draw=black,rounded corners=2mm, dotted, minimum width=15cm, minimum height=8.2cm, fit = (UBheur) (dummycheck2) (stopping) (vio2.north)] (Phase2)  {};

\node (p1) [above of=Phase1,xshift = 0.25cm, yshift = -0.4cm,text width=10cm] {\textbf{Phase one: Before branch-and-cut.}};
\node (p2) [above of=Phase2,xshift = -4.75cm, yshift = 3cm,text width=5cm] {\textbf{Phase two: Branch-and-cut.}};
\end{tikzpicture}
}
\caption{Flow chart of the two-stage decomposition algorithm.}%UB, $\nu$ and $(\bar{\zvar},\bar{\bvar},\bar{\nvar})$ denote upper bound of the SIP, the optimal objective value of the LP relaxation, and an optimal solution of the LP relaxation, respectively.
\label{fig: impl_flowchart1}
\end{center}
\end{figure}

%--%
\input{AppendBendersThree}
\input{AppendImplThree}
\input{AppendTable}
%\end{APPENDICES}
\clearpage

\bibliographystyle{informs2014} % outcomment this and next line in Case 1
%\bibliography{writeup_reference} % if more than one, comma separated

\end{document}
